# Supplementary material for: RASA: Replace Anyone, Say Anything -- A Training-Free Framework for Audio-Driven and Universal Portrait Video Editing
Source: arXiv:2503.11571 source file (2025-03-14)
Supplement: Supplementary file 1 [file X_suppl.tex]

% \clearpage
% \setcounter{page}{1}
% \maketitlesupplementary


% \section{Rationale}
% \label{sec:rationale}
% % 
% Having the supplementary compiled together with the main paper means that:
% % 
% \begin{itemize}
% \item The supplementary can back-reference sections of the main paper, for example, we can refer to \cref{sec:intro};
% \item The main paper can forward reference sub-sections within the supplementary explicitly (e.g. referring to a particular experiment); 
% \item When submitted to arXiv, the supplementary will already included at the end of the paper.
% \end{itemize}
% % 
% To split the supplementary pages from the main paper, you can use \href{https://support.apple.com/en-ca/guide/preview/prvw11793/mac#:~:text=Delete%20a%20page%20from%20a,or%20choose%20Edit%20%3E%20Delete).}{Preview (on macOS)}, \href{https://www.adobe.com/acrobat/how-to/delete-pages-from-pdf.html#:~:text=Choose%20%E2%80%9CTools%E2%80%9D%20%3E%20%E2%80%9COrganize,or%20pages%20from%20the%20file.}{Adobe Acrobat} (on all OSs), as well as \href{https://superuser.com/questions/517986/is-it-possible-to-delete-some-pages-of-a-pdf-document}{command line tools}.


% \paragraph{Compared baselines.} The proposed method is compared with several state-of-the-art video dubbing methods: 
% 1) Wav2Lip~\cite{wav2lip_2020} is widely recognized for its ability to produce realistic lip synchronization in videos through the use of a strong pre-trained discriminator dedicated to lip syncing. 
% 2) VideoReTalking~\cite{videoretalking_2022} achieves high-quality audio-driven lip synchronization for editing talking head videos by employing a method that includes expression neutralization, lip-sync generation, and enhancements that are aware of the speaker's identity.
% 3) DI-Net~\cite{dinet_2023} generates photorealistic and emotionally coherent talking face videos by utilizing a dual-encoder framework in conjunction with a system that focuses on facial action units.
% 4) TalkLip~\cite{talklip_2023} presents a novel contrastive learning method aimed at enhancing lip-speech synchronization, incorporating a transformer model to align audio with video while considering the overall temporal dependencies of the audio.
% 5) MuseTalk~\cite{musetalk_2024} generates lip-sync targets in a latent space encoded by a Variational Autoencoder, enabling high-fidelity talking face video generation with efficient inference.

% \begin{figure}
%     \centering
%     \includegraphics[width=0.8\linewidth]{pictures/ablation_pnpt.pdf}
%     \caption{\textbf{Ablation study for the temporal control injection timesteps $\tau_t$.} Temporal injection is crucial for ensuring temporal coherence and consistency.}
%     \label{fig:ablation_for_pnpt}
% \end{figure}

% \paragraph{Temporal control injection.} As illustrated in \Cref{fig:ablation_for_pnpt}, we configured the initial injection inversion timesteps to 0.0, 0.5, and 1.0 of the total denoising timesteps $T$. We observe that when $\tau=0.0T$, it indicates the absence of the temporal attention injection module, resulting in noticeable blurring or distortion during large-scale movements in the source-driven video. Additionally, as the temporal injection timesteps increase from 0.0 to 1.0, we notice that more background details are preserved, including the intricate features of the flag in this example.
